# Supplementary material for: Temporal localized states and square-waves in semiconductor micro-resonators with strong time-delayed feedback
Source: arXiv:2301.09400 source file (2023-04-26)
Supplement: Supplementary file 2 [file packages.tex]

\usepackage[utf8]{inputenc}
\usepackage{amsmath}
\usepackage{amsfonts}
\usepackage{amssymb}
\usepackage[english]{babel}
\usepackage[final]{graphicx} 
\usepackage{import}
%\usepackage{a4}
\usepackage{xr}
\usepackage{bm} %to write even greek letters in bold
\usepackage{tikz}
\usepackage{longtable,tabu}
\usepackage[european]{circuitikz}
\usepackage[output-decimal-marker={,}]{siunitx}
\usepackage{placeins}
\usepackage{diagbox}
\sisetup{separate-uncertainty}
\usepackage[colorlinks=true,linkcolor=black]{hyperref}
%\usepackage{hyperref}
\usepackage{subcaption}
\captionsetup[subfigure]{list=true, font=large, labelfont=bf, 
labelformat=brace, position=top}
\usepackage{amsmath}
\usepackage{tabu}
\usepackage{ifdraft}
\usepackage[backend=biber,sorting=none, style=alphabetic, natbib = true, maxbibnames=99]{biblatex}
\bibliography{Settings/lit.bib}
%\defbibheading{bibliography}{\section{Literatur}}
\usepackage[top=3cm,bottom=3cm]{geometry}
\setlength\parindent{0pt}
\usepackage{csquotes}
%\usepackage[onehalfspacing]{setspace}

\addto\extrasngerman{
	\let\subsectionautorefname\sectionautorefname
	\let\subsubsectionautorefname\sectionautorefname
}

\usepackage{chngcntr}
\counterwithin{figure}{section}
\counterwithin{table}{section}
\counterwithin{equation}{section}

\ifdraft{
	\usepackage{refcheck}
	\newcommand{\refcheckize}[1]{%
	  \expandafter\let\csname @@\string#1\endcsname#1%
	  \expandafter\DeclareRobustCommand\csname relax\string#1\endcsname[1]{%
	    \csname @@\string#1\endcsname{##1}\wrtusdrf{##1}}%
	  \expandafter\let\expandafter#1\csname relax\string#1\endcsname
	}
	\refcheckize{\autoref}
	\usepackage[german,colorinlistoftodos]{todonotes}
	\usepackage{draftwatermark}
	\SetWatermarkText{ENTFWURF}
	\SetWatermarkScale{5}
	\SetWatermarkColor[rgb]{0.7,0,0}
	\SetWatermarkLightness{0.9}
	\newcommand{\todoDiscuss}[1]{\todo[color=green!40]{#1}}
	\newcommand{\todoMissing}[1]{\todo[inline,color=red!40]{Fehlt noch: #1}}
	\newcommand{\todoNote}[1]{\todo[color=orange!40]{#1}}
	\newcommand{\todoMissingFigure}[1]{\missingfigure{#1}}
}{
	\newcommand{\todoDiscuss}[1]{\errmessage{Noch zu Diskutieren: #1}}
	\newcommand{\todoMissing}[1]{\errmessage{Fehlt noch: #1}}
	\newcommand{\todoNote}[1]{\errmessage{Noch zu tun: #1}}
	\newcommand{\todoMissingFigure}[1]{\errmessage{Bild Fehlt: #1}}
}




% maths

    \usepackage{siunitx}
    \numberwithin{equation}{section}   % Formelnummern entsprechen section (z.B. 1.1)
    \usepackage{braket} %Der Erwartungswert von $\braket{H}$ ist gleich $\braket{\psi|H|\psi}$
    \usepackage{dsfont} %Paket für doublestrokedinge, wie beispielsweise eine schöne mathbb 1. The command is \mathds{1}
    \usepackage{accents}    
    \usepackage{mathtools}
